# Supplementary material for: Millimeter Wave Analog Beamforming Codebooks Robust to Self-Interference
Source: arXiv:2105.13450 source file (2021-05-27)
Supplement: Supplementary file 1 [file sec-appendix.tex]

\appendices

\section{Test}
